# Supplementary material for: TorchGT: A Holistic System for Large-scale Graph Transformer Training
Source: arXiv:2407.14106 source file (2024-07-19)
Supplement: Supplementary file 1 [file 10_Appendix.tex]

% \appendix
%-------------------------------------------------------------------------------
\section{Artifact Description}
\label{sec_ad}
%-------------------------------------------------------------------------------

\subsection{Overview of Contributions and Artifacts}

\noindent\textbf{Paper's Main Contributions}. 
\begin{itemize}[leftmargin=*, itemsep=0pt, topsep=0pt, label=\ding{72}]
\item \SysName is the \textit{first} graph transformer system that facilitates efficient, scalable, and accurate training on large-scale graphs as well as universal graph learning tasks.

\item \SysName is the \textit{first} to identify the major challenges that hinder existing graph transformers from scaling to large graphs and explore the graph-specific optimization opportunities which are neglected previously.

\item We propose three key techniques to meet all design goals from algorithm and system co-design perspectives.

\item Experiments show \SysName achieves up to 62.7$\times$ speedup and near-linear scalability, supporting graph sequence lengths of up to millions.

\end{itemize}

\subsection{Artifact Identification}

This artifact appendix describes how to reproduce the main results in our paper. In our public repository, we provide the source code, related dataset and the instructions to run the code. Please refer to the README.md file for more details. For all experiments, we use two servers: \one Servers equipped with 8 GPUs (NVIDIA RTX 3090, each has 24GB GDDR6X Memory), one 32-thread CPU (AMD Threadripper PRO 3955WX) and 192GB DDR4 Memory. The intra-server communication (CPU-GPU and GPU-GPU) is based on PCIe 4.0 lanes. And the inter-server communication is achieved via 1Gps Ethernet. \two 2 servers each with 8 A100 GPUs (80GB) with NVLink and 200Gbps InfiniBand. \SysName is built on PyTorch 2.1.

\noindent\textbf{Program}: Python; Shell Script.

\noindent\textbf{Run-time environment}: Ubuntu 20.04 with Python 3.10, Pytorch 2.1, CUDA 12.0 and cuDNN 8.9.6. 

\noindent\textbf{Hardware}: Each 3090 server is equipped with dual-sockets 32-thread CPU (AMD Threadripper PRO 3955WX, 192GB DDR4 Memory) and 8 NVIDIA RTX 3090 GPUs (24GB memory).

\noindent\textbf{How much disk space is required (approximately)?} 300GB.

\noindent\textbf{Models and Datasets.} We choose two popular GNN models, which are most popular in graph transformer architectures: (1) Graphormer, (2) GT. For the Graphormer model, we have two variants: GPH$_{Large}$ and GPH$_{Slim}$. The learning rate begins at 0.0002, decays in a polynomial way and finally ends at $1e^{-9}$. The attention dropout rate is 0.5, input dropout rate is 0.1 and dropout rate for other layers is 0.3. 

We use five large-scale datasets in our evaluations which cover both graph-level and node-level tasks: (1) MalNet (graph-level), (2) ogbn-papers100m, (3) ogbn-products, (4) ogbn-arxiv and (5) Amazon.

% \noindent{\textbf{Malnet Preprocessing. }}
MalNet is the full version compared with MalNet-tiny. We construct the MalNet dataset from the original full dataset. We choose 5 classes of graphs including 
\texttt{benign}, \texttt{trojan}, \texttt{adware}, \texttt{downloader}, and \texttt{addisplay}, and select graphs with the largest number of vertices in each class. We also keep the graph number of each class relatively balanced and set the total graph number to 2$\times$ of Malnet-tiny.

\noindent\textbf{Expected Results.} \SysName should be far more faster than baselines such as \FlashGT, and is able to train large graphs compared with \RawGT, which incurrs out of memory on all datasets on 3090 server with 24GB.

\noindent\textbf{Expected Reproduction Time.} For the end-to-end experiments, it takes about 2 days to reproduce all experiments. For experiments on MalNet and ogbn-papers100M, the training time will take longer up to 22 hours for sequence length of 256K.

\subsection{Description}

For the complete description of the experiment workflow and results, we provide code and detailed documentation of \SysName in the following artifact repository: \url{https://anonymous.4open.science/r/TorchGT-83B2/}

\clearpage

% \subsection{Description}
